# Supplementary material for: Finer Grained Entity Typing with TypeNet
Source: arXiv:1711.05795 source file (2017-11-15)
Supplement: Supplementary file 1 [file appendix.tex]

\clearpage
\newpage

\appendix

\section{Appendix}
